# Supplementary material for: Experimental validation of a micromechanically-based compaction law for soft/hard grain mixtures
Source: arXiv:2111.01568 ancillary file (2021-11-02)
Supplement: Supplementary file 1 [file SM.pdf]

# supplementary material for: Experimental validation of a micromechanically-based compaction law for soft/hard grain mixtures

Manuel Cárdenas-Barrantes,[1,*] Jonathan Barés,[1,†] Mathieu Renouf,[1,‡] and Émilien Azéma[1,2,§]

[1] *Laboratoire de Mécanique et Génie Civil, UMR 5508 CNRS-University Montpellier, 34095 Montpellier, France*
[2] *Institut Universitaire de France (IUF), Paris, France*

(Dated: November 2, 2021)

## TENSOR COMPUTATION

From the displacement field $\vec{u}$, the deformation gradient tensor is computed as follow:

$$\vec{\vec{F}} = \vec{\nabla}\vec{u} + \vec{\vec{I}} \tag{1}$$

where $\vec{\vec{I}}$ is the second order identity tensor. The right Cauchy-Green strain tensor is then obtained from [1]:

$$\vec{\vec{C}} = \vec{\vec{F}}^T \vec{\vec{F}} \tag{2}$$

Physically, this tensor reflects the differences between the metrics of the deformed and undeformed bodies. It is related to the Green-Lagrangian strain tensor as [1]:

$$\vec{\vec{E}} = 1/2(\vec{\vec{C}} - \vec{\vec{I}}) \tag{3}$$

Under the small deformation assumption this last tensor turns out to be the strain tensor $\vec{\vec{\varepsilon}}$ classically used in elasticity theory. The von Mises measure of the right Cauchy-Green strain tensor is obtained from:

$$\mathcal{C} = \sqrt{\vec{\vec{C}} : \vec{\vec{C}}} \tag{4}$$

## CRITERION FOR JAMMING TRANSITION

The jamming transition corresponds with the transition of a granular system from a fluid-like to solid-like behavior. Many definitions of this transition exist associated with many experimental ways to detect it. In this study, we have chosen to consider that system transition when it can bear a non-negligible load. From the measurement accuracy of the force sensors, this load has been chosen to be $P_c = 1$ kPa. As shown in fig. 1, the so deduced packing fraction, $\phi_0$, at the jamming transition correspond with a transition at coordination $Z_c = 3.77 \pm 0.05$. Hence we can conclude that both methods are equivalent and correct since $Z_c$ is found between 3 and 4 and is close to 4, which corresponds with the fact that particles are slippery [2].

## SYSTEM PREPARATION AND REPEATABILITY

Due to the scanner size and resolution, the system we study is relatively small ($\sim 100$ particles). As such, it is more sensitive to initial conditions and sample preparation. To limit this effect, for each experiment, we paid specific attention to prepare the system as homogeneous as possible: we initially minimized the vicinity of the particles of the same size and the same nature. Also, the systems were prepared loose enough to observe the jamming transition after at least 10 compression steps, which lets some space for the system to rearrange and forget a bit the initial conditions.

As shown in fig. 2 for some softness ratio, we repeated the experiments 3 times. For a given softness ratio, the same tendency is always observed. So for the sake of simplicity, in this study, we present the results coming from one experiment for each softness ratio.

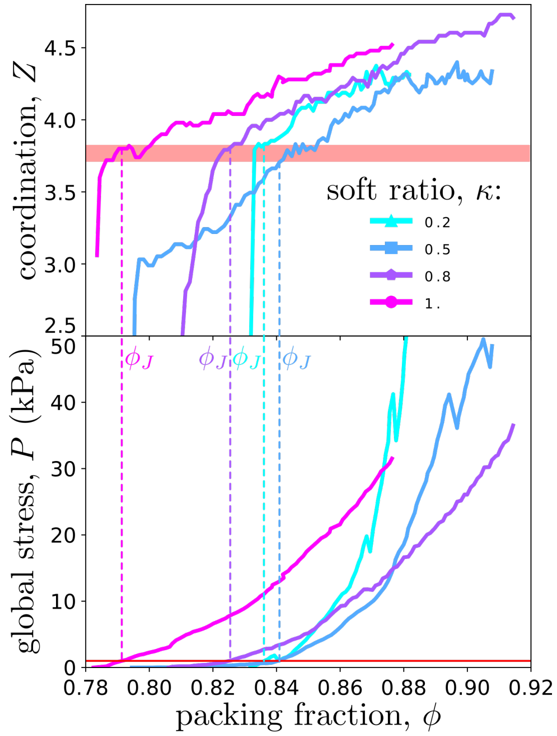


FIG. 1. top panel: evolution of the coordination number as a function of the packing fraction. bottom panel: evolution of the global pressure as a function of the packing fraction. An horizontal red line is plotted for $P = 1$ kPa. In both panels the different curves correspond with different soft to rigid number of particle ratio, $\kappa$.

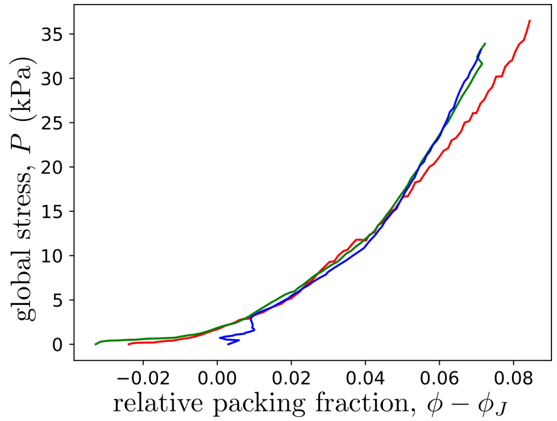


FIG. 2. Pressure as a function of the packing fraction for three independent experiments carried out with $\kappa = 0.8$. Experimental repeatability is very good.

## VON MISES STRAIN PROBABILITY DENSITY FUNCTIONS

## LINEARITY FOR $< l >$ *VS.* $\phi - \phi_J$

Assuming that $R$ is the radius of a circular particle, $L$ is the length of its contact with another particle or a wall, and $\delta$ is the loose of radius at the contact. Then the Hertz contact law [3] states that:

$$\frac{L}{2} = \sqrt{R\delta} \tag{5}$$

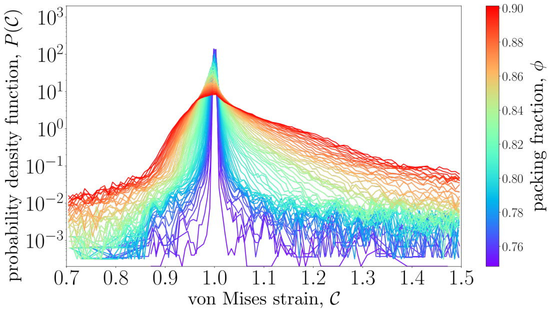


FIG. 3. Evolution of the probability density function of the von Mises strain in the soft particles along the compression as a function of the packing fraction. Data comes from an experiment with a softness ratio of 50%.

For a single contact on a particle, the relative contact length, $l$, can be written as:

$$l = \frac{L}{2\pi R} \tag{6}$$

To average over all particles and contacts we then multiply by the coordination number:

$$< l >= \frac{ZL}{2\pi R} \tag{7}$$

Also as stated in the letter and many other studies [4–8]:

$$Z = k\sqrt{\phi - \phi_J} \tag{8}$$

Then, we state the global strain as a function of the packing fraction:

$$\varepsilon = \frac{\phi - \phi_J}{\phi_J} \tag{9}$$

We also state that the global strain scale with $\delta$: $\varepsilon \sim \delta$. Typically in the case of a square network of particles of high $H0$, the strain is:

$$\varepsilon = 4\frac{\delta}{H0} \tag{10}$$

Plugging this scaling in eq.9, we get: $\delta \sim \phi - \phi_J$.
Using eq.8 we deduce that: $Z \sim \sqrt{\delta}$
So plugging this last relation in eq.7, we obtain: $< l >\sim L\sqrt{\delta}$
Finally using the scaling deduced from eq.5, we can state that:

$$< l >\sim \sqrt{\delta}\sqrt{\delta} = \delta \sim \phi - \phi_J \tag{11}$$

## UNIAXIAL COMPACTION MODEL FOR MIXED GRANULAR SYSTEMS

For the description of the compaction of cylindrical particles, the theoretical framework presented in [6, 7] is used and adapted to an uni-axial, plain-stress compaction. In this case the global pressure $P$ is related to the granular stress tensor through its $yy$ component by: $P = \sigma_{yy}$. This consideration, together with the fact that the volume $V_i$ of a cylinder is given by $V_i = \pi L d^2/4$, with $L$ the cylinder height, and $d$ its diameter leads to a slightly different micromechanical expression of $P$ in the form of [9]:

$$P \simeq \alpha_a \frac{Z\phi}{\pi}\sigma_l, \tag{12}$$

| $\kappa$ | $\phi_0$ | $\phi_{max}$ | $E^*$ (MPa) | $\Gamma$ |
|---|---|---|---|---|
| 0.2 | 0.836 | 0.88 | 2.67 | 4.38 |
| 0.5 | 0.841 | 0.93 | 1.00 | 3.57 |
| 0.8 | 0.826 | 0.96 | 0.62 | 3.54 |
| 1.0 | 0.791 | 0.97 | 0.50 | 3.05 |

TABLE I. Parameters used in Eq. (**??**) for the different mixture ratios. For all values of $\kappa$, $Z_0 = (3.77 \pm 0.05)$ and $\alpha = 0.7$.

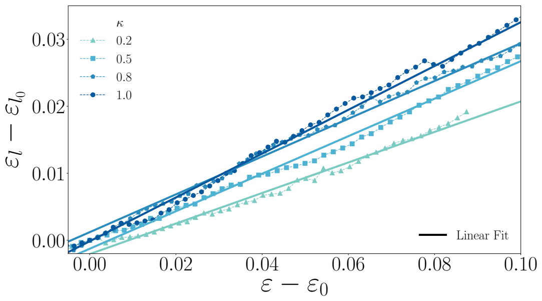


FIG. 4. Macroscopic volumetric strain $\epsilon$ as a function of the local strain $\epsilon_l$ at the small deformation domain for all $\kappa$ values.

where, in this case, $\sigma_l = \langle \ell \rangle \langle f_n \rangle / (Ld^2)$, and $\alpha_a$ a constant encompassing various microscopic parameters related to the anisotropy of the contact and force network, specific to uniaxial compression [9]. In practice $\alpha_a$ is hardly measurable experimentally. Nevertheless it has been shown that these anisotropies define the macroscopic friction $\mu_M$ of the assembly, leading to rewrite $\alpha_a \simeq 1 + \mu_M$ [9], with $\mu_M$ known to be close to 0.25 for an assembly of frictional disks, and assimilated here for cylinders. Then using the Hertz contact law, the mean contact pressure has the following form:

$$\sigma_l \simeq \frac{\pi}{4} E^* \varepsilon_l, \tag{13}$$

with $E^*$ the mean effective Young modulus, and $\varepsilon_l$ the mean local deformation. In mixtures, assuming the homogeneous distribution of the particles within the assemblies, and the equal mean number of contacts for the two types of particles, it comes that $E^* \approx E/(2\kappa(1-\nu^2))$. Finally, the linear trend between the local strain ($\varepsilon_l$) and its global counter part ($\varepsilon$) observed in fig. 4 show that the coefficient of proportionality ($\Gamma$) between these two quantities is well defined and depends on the softness ratio. Table I presents the values of $E^*$ and $\Gamma$ for the mixture ratios studied. With these new conditions, the compaction equation becomes the one presented in eq. 1 in the letter.


* manuel-antonio.cardenas-barrantes@umontpellier.fr
† jonathan.bares@umontpellier.fr
‡ Mathieu.Renouf@umontpellier.fr
§ emilien.azema@umontpellier.fr



[1] L. A. Taber, *Nonlinear theory of elasticity: applications in biomechanics* (World Scientific, 2004).
[2] M. van Hecke, Jamming of soft particles: geometry, mechanics, scaling and isostaticity, Journal of Physics: Condensed Matter **22**, 033101 (2009).
[3] L. D. Landau, E. M. Lifshitz, *et al.*, *Theory of elasticity*, Vol. 7 (Pergamon Press, Oxford New York, 1986).
[4] B. Andreotti, Y. Forterre, and O. Pouliquen, *Granular media: between fluid and solid* (Cambridge University Press, 2013).
[5] T.-L. Vu, J. Barés, S. Mora, and S. Nezamabadi, Numerical simulations of the compaction of assemblies of rubberlike particles: A quantitative comparison with experiments, Physical Review E **99**, 062903 (2019).
[6] D. Cantor, M. Cárdenas-Barrantes, I. Preechawuttipong, M. Renouf, and É. Azéma, Compaction model for highly deformable particle assemblies, Physical Review Letters **124**, 208003 (2020).
[7] M. Cárdenas-Barrantes, D. Cantor, J. Barés, M. Renouf, and E. Azéma, Compaction of mixtures of rigid and highly deformable particles: A micromechanical model, Physical Review E **102**, 032904 (2020).
[8] M. Cárdenas-Barrantes, D. Cantor, J. Barés, M. Renouf, and E. Azéma, Micromechanical description of the compaction of soft pentagon assemblies, Physical Review E **103**, 062902 (2021).

[9] L. Rothenburg and R. J. Bathurst, Analytical study of induced anisotropy in idealized granular materials, Geotechnique **39**, 601 (1989).
